# Supplementary material for: Computational study of the effects of density, fuel content, and moisture content on smoldering propagation of cellulose and hemicellulose mixtures
Source: arXiv:1806.08396 ancillary file (2018-06-21)
Supplement: Supplementary file 1 [file mulky-smoldering-supplementary_material.pdf]

# Supplementary Material for "Computational study of the effects of density, fuel content, and moisture content on smoldering propagation of cellulose and hemicellulose mixtures"

Tejas Chandrashekhar Mulky[a], Kyle E. Niemeyer[a,*]

[a]*School of Mechanical, Industrial, and Manufacturing Engineering*
*Oregon State University, Corvallis, OR 97331, USA*

**Abstract**

This Supplementary Material contains a description of the experimental setup used to provide validation data, the values of kinetic parameters used in the model, and a grid convergence study.

## 1. Details about the experimental set-up

The experiments were conducted on four cellulose and hemicellulose mixtures with varying density and compositions [1]. The cellulose content was varied from 100% to 25% by mass with a decrement of 25% the remaining portion being hemicellulose where the density of the fuels were 188.75 kg/m$^3$, 237.14 kg/m$^3$, 364.28 kg/m$^3$, and 527.71 kg/m$^3$, respectively. The fuel samples were held in a rector box with the following dimensions: $20 \times 20 \times 10$ cm. The reactor box was made from fiberboard. The top surface was open to the atmosphere. The cellulose used in the experiments was $\alpha$-cellulose purchased from Sigma-Aldrich (CAS no: 9004-34-6) and hemicellulose used in the experiments was glucomannon purchased from Nutricost. The fuel was ignited using a 20 W cartridge heater with a diameter of 64 mm. The cartridge heater was placed at the center of the reactor box. Type-K thermocouples were placed at 0, 2.5, 5, and 7.5 cm from the top surface.

## 2. Kinetic parameters for cellulose and hemicellulose

$$\text{Cellulose} \cdot v_{w,dr}\text{H}_2\text{O} \longrightarrow \text{Cellulose} + v_{w,dr}\text{H}_2\text{O}\,(\text{g}) \tag{1}$$

$$\text{Cellulose} \longrightarrow v_{\alpha,cp}\alpha{-}\text{Char}_c + v_{g,cp}\text{Gas} \tag{2}$$

$$\text{Cellulose} + v_{O_2,co}\text{O}_2 \longrightarrow v_{\beta,co}\beta{-}\text{Char}_c + v_{g,co}\text{Gas} \tag{3}$$

$$\alpha\text{-Char}_c + v_{O_2,c\alpha o}\,\text{O}_2 \longrightarrow v_{a,c\alpha o}\text{Ash}_c + v_{g,c\alpha o}\text{Gas} \tag{4}$$

$$\beta\text{-Char}_c + v_{O_2,c\beta o}\text{O}_2 \longrightarrow v_{a,c\beta o}\text{Ash}_c + v_{g,c\beta o}\text{Gas} \tag{5}$$

$$\text{Hemicellulose} \cdot v_{w,dr}\text{H}_2\text{O} \longrightarrow \text{Hemicellulose} + v_{w,dr}\text{H}_2\text{O}\,(\text{g}) \tag{6}$$

$$\text{Hemicellulose} \longrightarrow v_{\alpha,hp}\alpha{-}\text{Char}_h + v_{g,hp}\text{Gas} \tag{7}$$

$$\text{Hemicellulose} + v_{O_2,ho}\text{O}_2 \longrightarrow v_{\beta,ho}\beta{-}\text{Char}_h + v_{g,ho}\text{Gas} \tag{8}$$

$$\alpha\text{-Char}_h + v_{O_2,h\alpha o}\text{O}_2 \longrightarrow v_{a,h\alpha o}\text{Ash}_h + v_{g,h\alpha o}\text{Gas} \tag{9}$$

$$\beta\text{-Char}_h + v_{O_2,h\beta o}\text{O}_2 \longrightarrow v_{a,h\beta o}\text{Ash}_h + v_{g,h\beta o}\text{Gas} \tag{10}$$

*Corresponding author
*Email address:* `kyle.niemeyer@oregonstate.edu` (Kyle E. Niemeyer)

where $v$ is the stoichiometric coefficient; $\alpha$ and $\beta$ indicate char produced from fuel pyrolysis and fuel oxidation reactions, respectively; and subscripts $w$, $g$, $O_2$, $a$, $c$, $h$, $dr$, $o$, $p$, $\alpha o$, $\beta o$ are water, gas, oxygen, ash, cellulose, hemicellulose, drying, oxidation, pyrolysis, $\alpha$-char oxidation, and $\beta$-char oxidation, respectively.

Table 1 lists the reaction parameters for the chemical kinetic schemes used in the simulation, obtained from Huang and Rein [2].

Table 1: Kinetic and and stoichiometric parameters for cellulose and hemicellulose models from Huang and Rein [3].

| Reaction number | Reaction | Cellulose<br>$\log Z$<br>$\log \mathrm{s}^{-1}$ | $E$<br>kJ/mol | $\Delta H$<br>MJ/kg | $n$<br>– | $n_{O_2}$<br>– |
|---|---|---|---|---|---|---|
| (1) | Drying | 8.12 | 67.8 | 2.26 | 2.37 | – |
| (2) | Pyrolysis | 11.7 | 156 | 0.5 | 1 | – |
| (3) | Oxidation | 24.2 | 278 | -28.2 | 1.73 | 0.74 |
| (4) | $\beta$-char oxidation | 7.64 | 120 | -28.8 | 1.25 | 0.89 |
| (5) | $\alpha$-char oxidation | 12.2 | 177 | -27.8 | 0.93 | 0.52 |
| Reaction Number | Reaction | Hemicellulose<br>$\log Z$<br>$\log \mathrm{s}^{-1}$ | $E$<br>kJ/mol | $\Delta H$<br>MJ/kg | $n$<br>– | $n_{O_2}$<br>– |
| (6) | Drying | 8.12 | 67.8 | 2.26 | 2.37 | – |
| (7) | Pyrolysis | 6.95 | 93.8 | 0.5 | 0.98 | – |
| (8) | Oxidation | 20.2 | 294 | -20.9 | 0.47 | 0.11 |
| (9) | $\beta$-char oxidation | 7.64 | 120 | -28.8 | 1.25 | 0.89 |
| (10) | $\alpha$-char oxidation | 12.2 | 177 | -27.8 | 0.93 | 0.52 |

## 3. Grid convergence study

We performed a grid convergence study, as shown in Figure 1 for the smoldering wave propagation speed as a function of cell size. Our simulations were performed using a uniform cell size of $1 \times 10^{-5}$ m, and as Fig. 1 shows reducing the cell size further leads to negligible change in the propagation speed.

## References


[1] B. D. Smucker, D. A. Cowan, D. L. Blunck, Personal communication, 15 February 2018 (2018).

[2] X. Huang, G. Rein, Thermochemical conversion of biomass in smouldering combustion across scales: The roles of heterogeneous kinetics, oxygen and transport phenomena, Bioresource Technology 207 (2016) 409–421. doi:10.1016/j.biortech.2016.01.027.

[3] X. Huang, G. Rein, Downward spread of smouldering peat fire : the role of moisture , density and oxygen supply, Internation Journal of Wildland Fire 26 (2017) 907–918. doi:10.1071/WF16198.

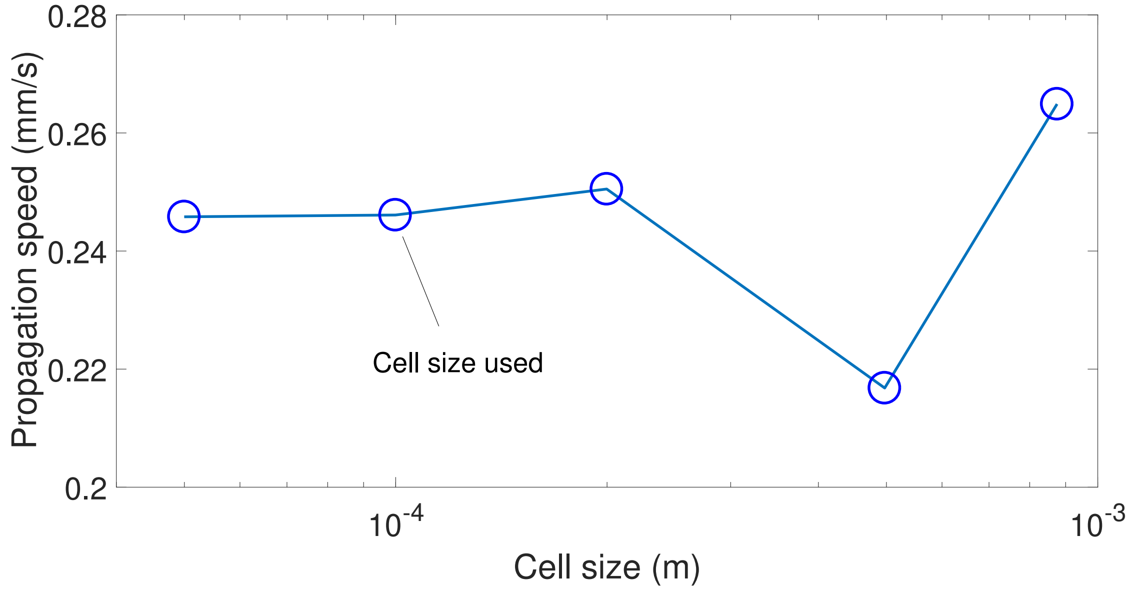


Figure 1: Impact of refining the uniform grid size on calculated propagation speed of the smoldering wave.
